# Supplementary material for: CAST: Clustering Self-Attention using Surrogate Tokens for Efficient Transformers
Source: arXiv:2402.04239 source file (2024-02-06)
Supplement: Supplementary file 3 [file speedmemory_results.tex]

\begin{table*}[h!]
    \centering
    \resizebox{\textwidth}{!}{ \begin{tabular}{l|cccc|cccc}
        \toprule
        \multirow{2}{*}{\textbf{Model}} & \multicolumn{4}{c}{Steps Per Second $\uparrow$} & \multicolumn{4}{|c}{Peak Memory Usage $\downarrow$} \\
        & 1K & 2K & 3K & 4K & 1K & 2K & 3K & 4K \\
        \midrule
        Transformer \cite{vaswani2017attention} & 1.0 & 1.0 & 1.0 & 1.0 & 1.0 & 1.0 & 1.0 & 1.0\\
        \midrule
        $\text{Reformer}^\dag$ \cite{reformer} & 0.5 & 0.4 & 0.7 & 0.8 & 0.56 & 0.37 & 0.28 & 0.24\\
        $\text{Sinkhorn Trans.}^\dag$ \cite{sinkhornTransformer} & 1.1 & 1.6 & 2.9 & 3.8 & 0.55 & 0.31 & 0.21 & 0.16\\
        $\text{Performer}^\dag$  \cite{performer}& \textbf{1.2} & 1.9 & 3.8 & 5.7 & 0.44 & 0.22 & 0.15 & 0.11 \\
        Luna-16 \cite{luna} & \textbf{1.2} & 1.8 & 3.7 & 5.5 & 0.44 & 0.23 & 0.17 &\textbf{0.10} \\
        S4 \cite{gu2022efficientlys4} & - & - & - & 4.8 & - & - & - & 0.14 \\
        MEGA \cite{ma2023mega} & - & - & - & 2.9 & - & - & - & 0.31 \\
        MEGA-Chunk \cite{ma2023mega} & - & - & - & 5.5 & - & - & - & 0.13 \\
        CAST (Ours) & 0.90 & \textbf{3.25} & \textbf{4.48} & \textbf{6.16} & \textbf{0.34} & \textbf{0.19} & \textbf{0.13} & \textbf{0.10}\\
        \bottomrule
    \end{tabular}}
    \caption{Speed and Memory experiment of the LRA Benchmark, the Transformer, and CAST was created using the same hyperparameters. A batch size of 32 was used and CAST uses a constant cluster size of 200. Speed and Memory increase/decrease are reported relative to the results of the original Transformer architecture. Models annotated with the $\dag$ symbol had their relative speed and memory taken in the LRA dataset \cite{tay2020long}. %Other results were taken from their respective papers.
    }
    \label{tab:lra_speed}
\end{table*}
