# Supplementary material for: CAST: Clustering Self-Attention using Surrogate Tokens for Efficient Transformers
Source: arXiv:2402.04239 source file (2024-02-06)
Supplement: Supplementary file 5 [file visual_analysis_extra.tex]

\begin{figure}[h!]
\centering
    \begin{subfigure}{0.30\textwidth}
    \includegraphics[width=\textwidth]{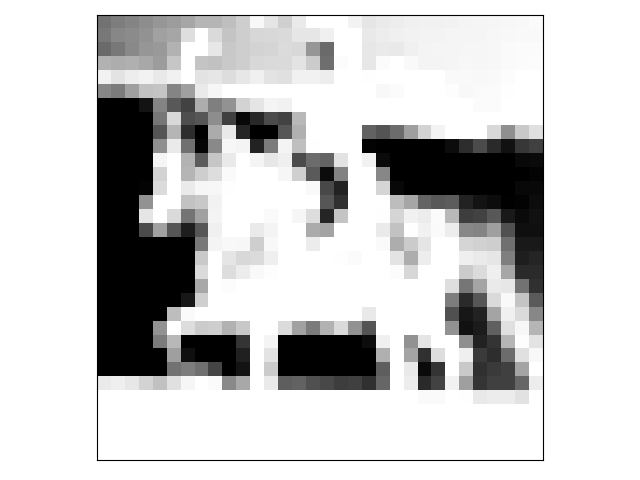}
    \caption{Example Image of the LRA \textbf{Image} task.}
    \label{fig:example-image-1}
    \end{subfigure}
    \begin{subfigure}{0.30\textwidth}
    \includegraphics[width=\textwidth]{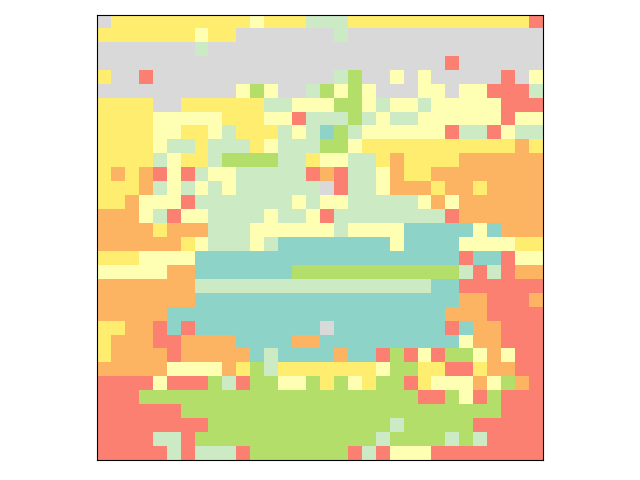}
    \caption{Clustered Image, $N_c=8$, Layer 1.}
    \label{fig:clustered-1}
    \end{subfigure}
    \begin{subfigure}{0.30\textwidth}
    \includegraphics[width=\textwidth]{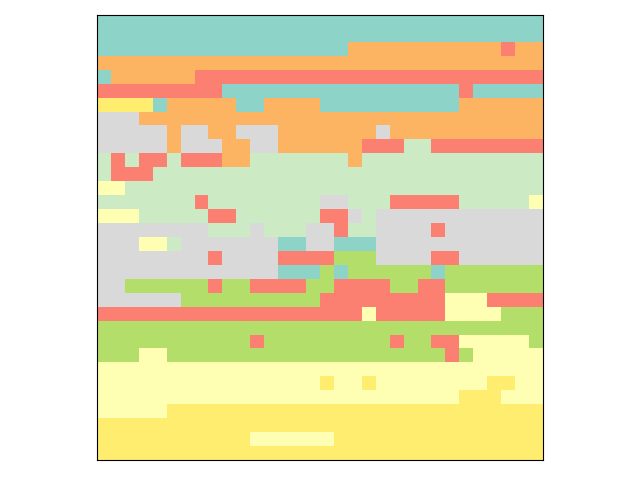}
    \caption{Clustered Image, $N_c=8$, Layer 2.}
    \label{fig:clustered-2}
    \end{subfigure}
    \\\vspace{1em}
    \begin{subfigure}{\textwidth}
        \centering
        \begin{subfigure}{0.22\textwidth}
        \includegraphics[width=\textwidth]{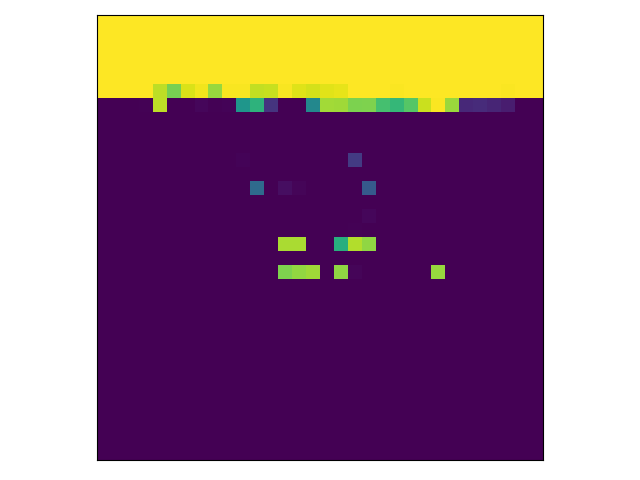}
        \end{subfigure}
        \begin{subfigure}{0.22\textwidth}
        \includegraphics[width=\textwidth]{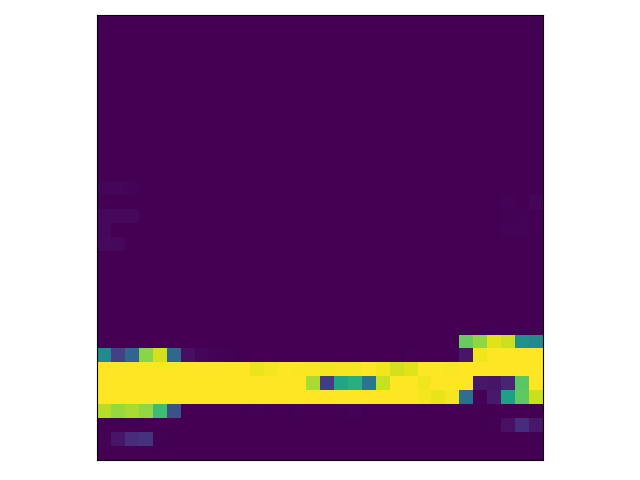}
        \end{subfigure}
        \begin{subfigure}{0.22\textwidth}
        \includegraphics[width=\textwidth]{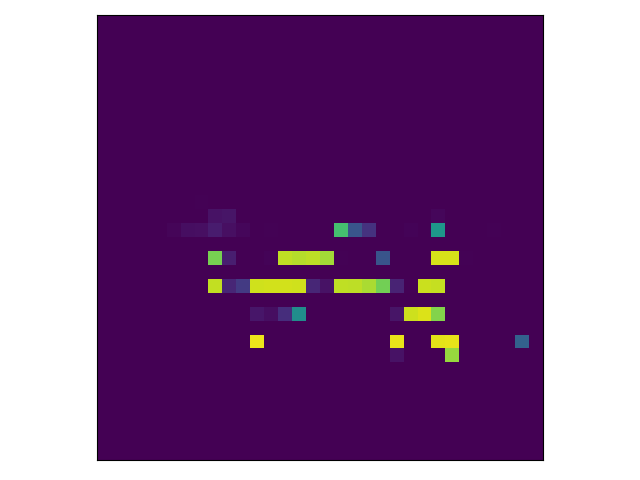}
        \end{subfigure}
        \begin{subfigure}{0.22\textwidth}
        \includegraphics[width=\textwidth]{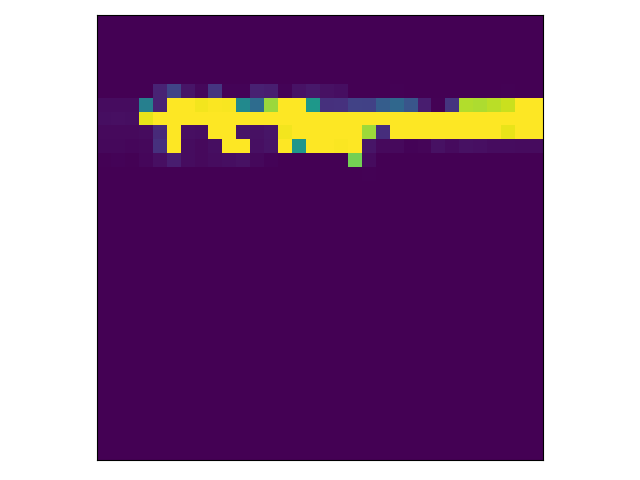}
        \end{subfigure}
        \\\vspace{1em}
        \begin{subfigure}{0.22\textwidth}
        \includegraphics[width=\textwidth]{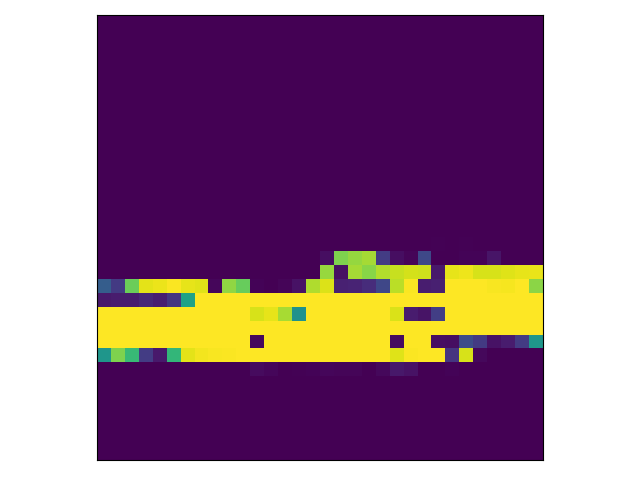}
        \end{subfigure}
        \begin{subfigure}{0.22\textwidth}
        \includegraphics[width=\textwidth]{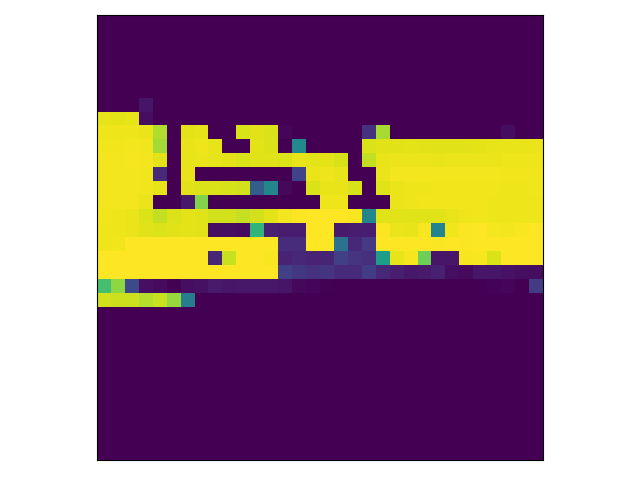}
        \end{subfigure}
        \begin{subfigure}{0.22\textwidth}
        \includegraphics[width=\textwidth]{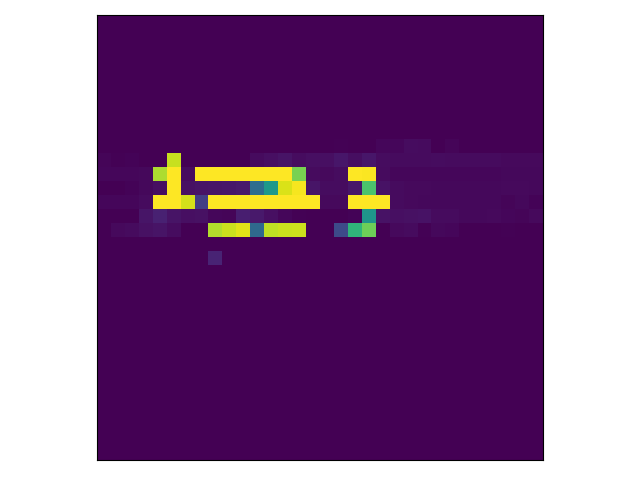}
        \end{subfigure}
         \begin{subfigure}{0.22\textwidth}
        \includegraphics[width=\textwidth]{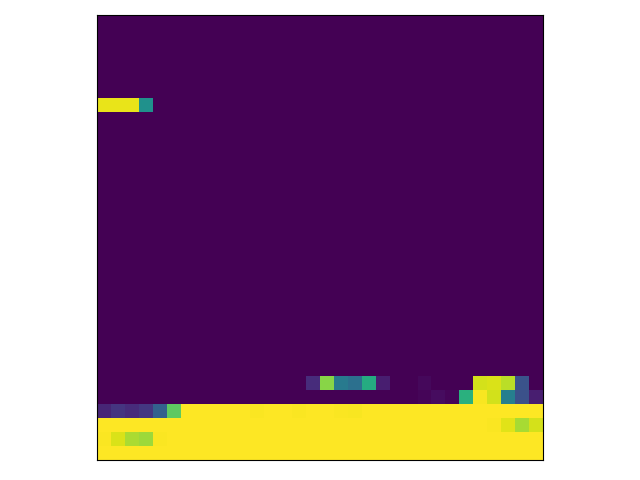}
        \end{subfigure}
    \caption{Scores of $\textbf{A}_g$ per cluster for Layer 1 of a CAST model trained on the \textbf{Image} task of LRA.}
    \label{}
    \end{subfigure}
    \\
    \begin{subfigure}{\textwidth}
        \centering
        \begin{subfigure}{0.22\textwidth}
        \includegraphics[width=\textwidth]{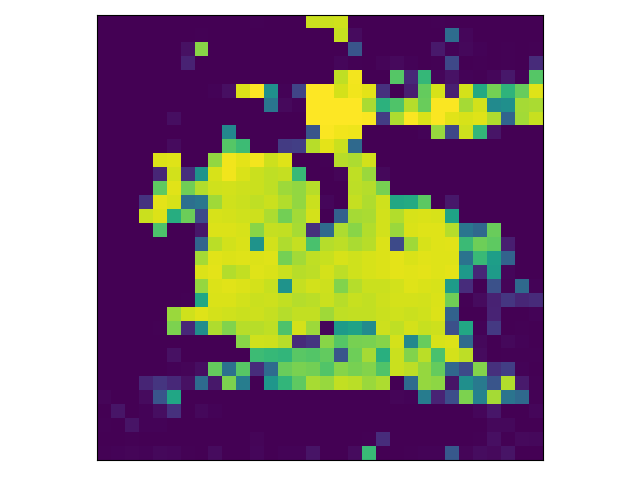}
        \end{subfigure}
        \begin{subfigure}{0.22\textwidth}
        \includegraphics[width=\textwidth]{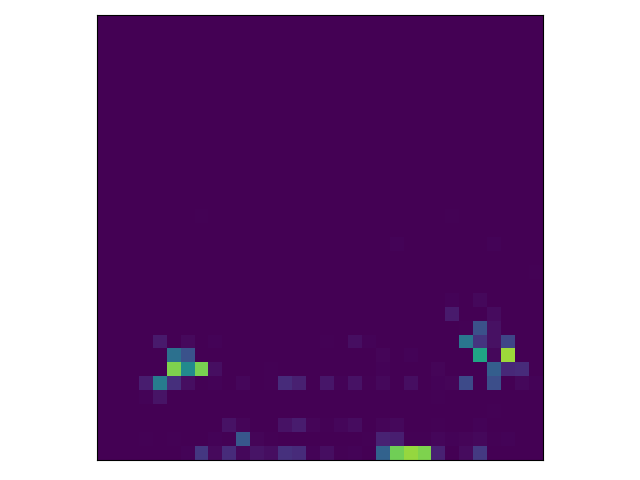}
        \end{subfigure}
        \begin{subfigure}{0.22\textwidth}
        \includegraphics[width=\textwidth]{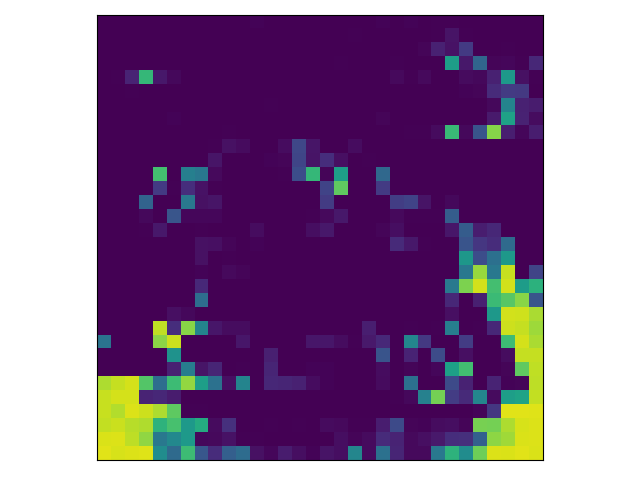}
        \end{subfigure}
        \begin{subfigure}{0.22\textwidth}
        \includegraphics[width=\textwidth]{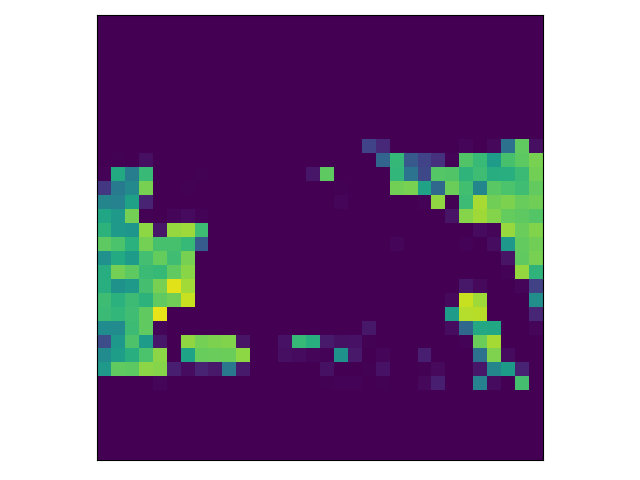}
        \end{subfigure}
        \\\vspace{1em}
        \begin{subfigure}{0.22\textwidth}
        \includegraphics[width=\textwidth]{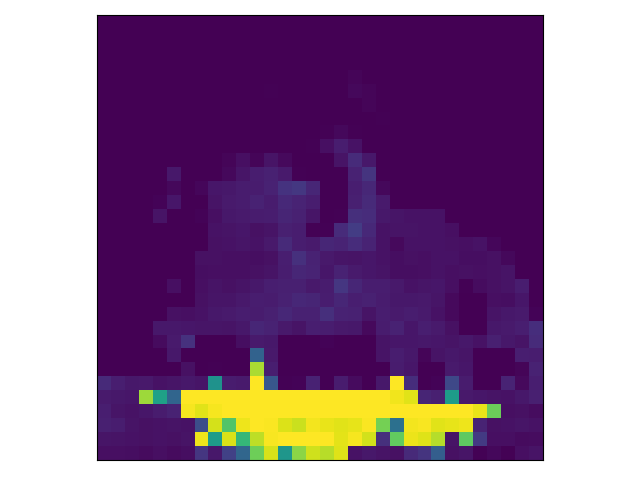}
        \end{subfigure}
        \begin{subfigure}{0.22\textwidth}
        \includegraphics[width=\textwidth]{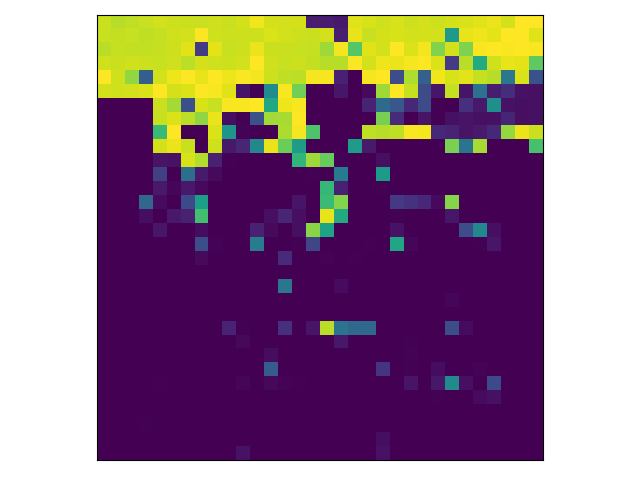}
        \end{subfigure}
        \begin{subfigure}{0.22\textwidth}
        \includegraphics[width=\textwidth]{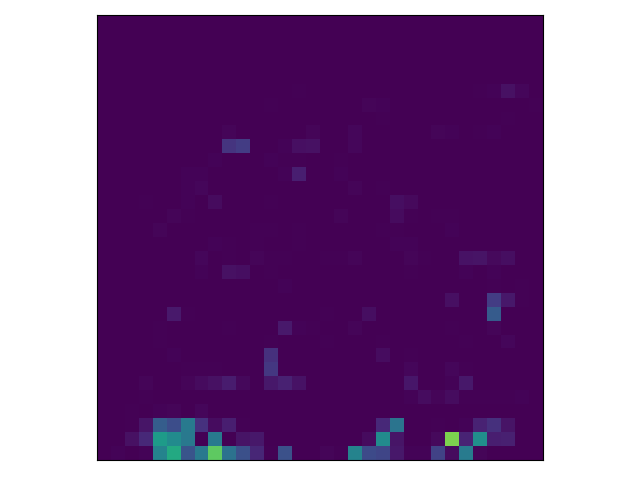}
        \end{subfigure}
         \begin{subfigure}{0.22\textwidth}
        \includegraphics[width=\textwidth]{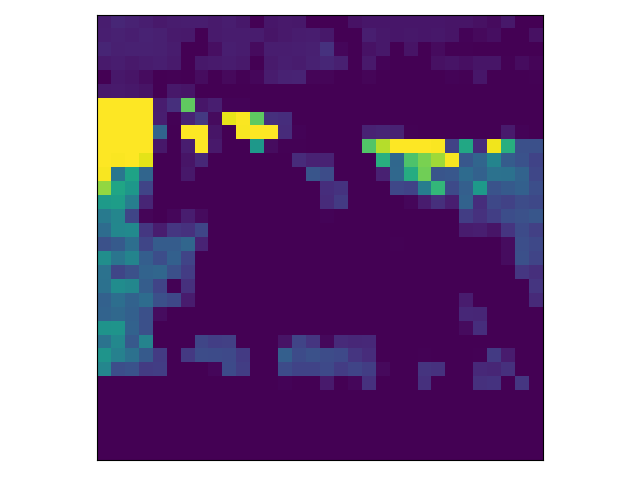}
        \end{subfigure}
    \caption{Scores of $\textbf{A}_g$ per cluster for Layer 2 of a CAST model trained on the \textbf{Image} task of LRA.}
    \label{fig:horse-vis}
    \end{subfigure}
    \caption{A visualization learned clusters in different layers of CAST. Here, the clustered image is from the \textbf{Image} of LRA, depicting a horse with a rider.}
\end{figure}
